# Supplementary material for: Highly Available Transactions: Virtues and Limitations (Extended Version)
Source: arXiv:1302.0309 source file (2013-10-07)
Supplement: Supplementary file 1 [file availability-appendix.tex]

\section{Availability}

\begin{definition}[$K$-Availability]
A system provides $K$-Availability if
\end{definition}

\begin{definition}[High Availability]
A system provides High Availability if it provides $1$-Availability.
\end{definition}

\begin{definition}[Sticky $K$-Availability]
A system provides Sticky $K$-Availability if 
\end{definition}

\begin{definition}[Sticky High Availability]
A system provides Sticky High Availability if it provides Sticky
$1$-Availability.
\end{definition}

\begin{definition}[Availability Strength]
An availability model $M_1$ is \textit{more available} than another
availability model $M_2$ if, whenever $M_2$ is satisfied, $M_1$ is
satisfied, and there is at least one configuration under which $M_1$
is satisfied but $M_2$ is not. If $M_1$ is more available than $M_2$,
then $M_2$ is \textit{less available} than $M_1$.
\end{definition}

\begin{observation}
Majority availability is less available than high sticky availability.
\end{observation}
